# Supplementary material for: Unsupervised Learning for Robust Fitting:A Reinforcement Learning Approach
Source: arXiv:2103.03501 source file (2021-03-05)
Supplement: Supplementary file 1 [file 06_Supp.tex]

% \clearpage
\section{Extension of the algorithm to quasi-convex residual cases}
This experiment demonstrates that our proposed method performs favorably for fitting problems with \textit{quasi-convex residuals}.
One of the common applications is homography fitting. Given a set of putative correspondences $\cX=\{(\bu_i, \bv_i)\}_{i=1}^N$, we estimate the homography matrix $\btheta \in \bbR^{3 \times 3}$. The residual is of the form:
\begin{equation*}
%r_{i}(\btheta) = \frac{A_{i}^T\btheta_{1:2} - b_{i}}{c_{i}^T\btheta - d_{i}},
r_{i}(\btheta) = \frac{||(\btheta_{1:2} - \bv_{i}\btheta_{3})\hat{\bu}_i||}{\btheta_{3}\hat{\bu}_i},
%r(\btheta) = \frac{p(\btheta)}{q(\btheta)},
\end{equation*}
where $\hat{\bu}_i = [\bu_i^{T} \hspace{2mm} 1]^{T}$, $\btheta_{1:2}$ is the first 2 rows of $\btheta$, and $\btheta_{3}$ is the last row of $\btheta$.
For this experiment, the state encoding $h(\bx_i)$, where $\bx_i = [\bu_i, \bv_i]$ discussion in Eq.(10) is chosen to be
\begin{equation*}
     h(\bx_i) = [\bu_i^T \;\; \bv_i^T].
\end{equation*}

We compare our algorithm with other methods as described in the main paper. We conduct our experiment in one sequence of KITTI dataset \cite{KittiData}. We compute and match SIFT keypoints using VLFeat toolbox. The inlier threshold is chosen as $\epsilon = 0.03$. As shown in Fig.~\ref{fig:realHomo}, our method generally achieves higher consensus size, compared to ULCM. When compared to RANSAC, despite the fact that our spread is larger, we have a smaller variance and higher median consensus size. This means that our method has much higher concentration on good results (with small tail to the distribution: \textit{only rarely} producing poor results).

\begin{figure}[ht]
      \centering
      \includegraphics[width=1\linewidth]{tex/figures/homoresult.pdf}
      \caption{Homography ftting on KITTI dataset}
      \label{fig:realHomo}
      \vspace{-3mm}
\end{figure}

\section{The role of Local Tree Refinement}
Fig.~\ref{fig:ablation} plots the consensus size in 2D Line Fitting experiment before and after applying refinement (Section 3.6 in the main paper). All results are obtained by running 100 times. Even though our RL based method performs competitively, the refinement process slightly improves the results. Note especially the performance of local refinement for outlier rates $>25\%$.  

%As can be seen, the results provided by our network is competitive even before performing local refinement.
\begin{figure}[ht]
      \centering
      \includegraphics[width=0.9\linewidth]{tex/figures/ablation.png}
      \caption{Consensus size of our proposed method, before and after refinement, in 2D line fitting experiment.}
      \label{fig:ablation}
      \vspace{-3mm}
\end{figure}
